# Supplementary material for: Closure Relations for Shallow Granular Flows from Particle Simulations
Source: arXiv:1108.5033 source file (2011-08-25)
Supplement: Supplementary file 1 [file Appendix2.tex]

%%%%%%%%%%%%%%%%%%%%%%%%%%%%%%%%%%%%%%%%%%%%%%%%%%%
\subsection{Parameters of the depth-averaged model}\label{sec:depthaveraging}
%%%%%%%%%%%%%%%%%%%%%%%%%%%%%%%%%%%%%%%%%%%%%%%%%%%

\begin{figure}[tbp]
% generated by laprint.m
%
\begin{psfrags}%
\psfragscanon%
%
% text strings:
\psfrag{s01}[t][t]{\fontsize{10}{15}\fontseries{m}\mathversion{normal}\fontshape{n}\selectfont \color[rgb]{0,0,0}\setlength{\tabcolsep}{0pt}\begin{tabular}{c}$\theta$\end{tabular}}%
\psfrag{s02}[b][b]{\fontsize{10}{15}\fontseries{m}\mathversion{normal}\fontshape{n}\selectfont \color[rgb]{0,0,0}\setlength{\tabcolsep}{0pt}\begin{tabular}{c}$\bar\rho/\rho_p$\end{tabular}}%
\psfrag{s05}[l][l]{\fontsize{10}{15}\fontseries{m}\mathversion{normal}\fontshape{n}\selectfont \color[rgb]{0,0,0}$\lambda=1/2$}%
\psfrag{s06}[l][l]{\fontsize{10}{15}\fontseries{m}\mathversion{normal}\fontshape{n}\selectfont \color[rgb]{0,0,0}$\lambda=2$}%
\psfrag{s07}[l][l]{\fontsize{10}{15}\fontseries{m}\mathversion{normal}\fontshape{n}\selectfont \color[rgb]{0,0,0}$\lambda=1$}%
\psfrag{s08}[l][l]{\fontsize{10}{15}\fontseries{m}\mathversion{normal}\fontshape{n}\selectfont \color[rgb]{0,0,0}$\lambda=5/6$}%
\psfrag{s09}[l][l]{\fontsize{10}{15}\fontseries{m}\mathversion{normal}\fontshape{n}\selectfont \color[rgb]{0,0,0}$\lambda=2/3$}%
\psfrag{s10}[l][l]{\fontsize{10}{15}\fontseries{m}\mathversion{normal}\fontshape{n}\selectfont \color[rgb]{0,0,0}$\lambda=1/2$}%
\psfrag{s12}[][]{\fontsize{10}{15}\fontseries{m}\mathversion{normal}\fontshape{n}\selectfont \color[rgb]{0,0,0}\setlength{\tabcolsep}{0pt}\begin{tabular}{c} \end{tabular}}%
\psfrag{s13}[][]{\fontsize{10}{15}\fontseries{m}\mathversion{normal}\fontshape{n}\selectfont \color[rgb]{0,0,0}\setlength{\tabcolsep}{0pt}\begin{tabular}{c} \end{tabular}}%
%
% axes font properties:
\fontsize{10}{15}\fontseries{m}\mathversion{normal}%
\fontshape{n}\selectfont%
%
% xticklabels:
\psfrag{x01}[t][t]{20}%
\psfrag{x02}[t][t]{21}%
\psfrag{x03}[t][t]{22}%
\psfrag{x04}[t][t]{23}%
\psfrag{x05}[t][t]{24}%
\psfrag{x06}[t][t]{25}%
\psfrag{x07}[t][t]{26}%
\psfrag{x08}[t][t]{27}%
\psfrag{x09}[t][t]{28}%
%
% yticklabels:
\psfrag{v01}[r][r]{0.52}%
\psfrag{v02}[r][r]{0.53}%
\psfrag{v03}[r][r]{0.54}%
\psfrag{v04}[r][r]{0.55}%
\psfrag{v05}[r][r]{0.56}%
\psfrag{v06}[r][r]{0.57}%
\psfrag{v07}[r][r]{0.58}%
\psfrag{v08}[r][r]{0.59}%
\psfrag{v09}[r][r]{0.6}%
\psfrag{v10}[r][r]{0.61}%
\psfrag{v11}[r][r]{0.62}%
%
% Figure:
\resizebox{8cm}{!}{\includegraphics{ha_Nu_2_3_4_5_6.matlab.eps}}%
\end{psfrags}%
%
% End ha_Nu_2_3_4_5_6.matlab.tex

%\input{FiguresMatlab/ha_Nu_5.matlab.tex}
\caption{Mean particle volume fraction $\bar\rho/\rho_p$ for varying approximated height $H=20, 30, 40$, inclination $\theta$ and roughness $\lambda$. Dashed line connects the values for $\lambda=1$, $H=40$. For thick flows, the volume fraction nearly collapses onto a function of the inclination, with a small dependence on the flow height. 
%Volume fractions remains almost constant in depth for all steady cases.%The particle volume fraction decreases independent of height for increasing chute angle.
}
\label{fig:Nu}
\end{figure} 

\begin{figure}[htbp]
%\input{FiguresMatlab/ha_alpha_5.matlab.tex}
% generated by laprint.m
%
\begin{psfrags}%
\psfragscanon%
%
% text strings:
\psfrag{s01}[t][t]{\fontsize{10}{15}\fontseries{m}\mathversion{normal}\fontshape{n}\selectfont \color[rgb]{0,0,0}\setlength{\tabcolsep}{0pt}\begin{tabular}{c}$\theta$\end{tabular}}%
\psfrag{s02}[b][b]{\fontsize{10}{15}\fontseries{m}\mathversion{normal}\fontshape{n}\selectfont \color[rgb]{0,0,0}\setlength{\tabcolsep}{0pt}\begin{tabular}{c}$\alpha$\end{tabular}}%
\psfrag{s05}[l][l]{\fontsize{8}{12}\fontseries{m}\mathversion{normal}\fontshape{n}\selectfont \color[rgb]{0,0,0}$\lambda=0$}%
\psfrag{s06}[l][l]{\fontsize{8}{12}\fontseries{m}\mathversion{normal}\fontshape{n}\selectfont \color[rgb]{0,0,0}$\lambda=2$}%
\psfrag{s07}[l][l]{\fontsize{8}{12}\fontseries{m}\mathversion{normal}\fontshape{n}\selectfont \color[rgb]{0,0,0}$\lambda=1$}%
\psfrag{s08}[l][l]{\fontsize{8}{12}\fontseries{m}\mathversion{normal}\fontshape{n}\selectfont \color[rgb]{0,0,0}$\lambda=5/6$}%
\psfrag{s09}[l][l]{\fontsize{8}{12}\fontseries{m}\mathversion{normal}\fontshape{n}\selectfont \color[rgb]{0,0,0}$\lambda=2/3$}%
\psfrag{s10}[l][l]{\fontsize{8}{12}\fontseries{m}\mathversion{normal}\fontshape{n}\selectfont \color[rgb]{0,0,0}$\lambda=1/2$}%
\psfrag{s11}[l][l]{\fontsize{8}{12}\fontseries{m}\mathversion{normal}\fontshape{n}\selectfont \color[rgb]{0,0,0}$\lambda=0$}%
\psfrag{s13}[][]{\fontsize{10}{15}\fontseries{m}\mathversion{normal}\fontshape{n}\selectfont \color[rgb]{0,0,0}\setlength{\tabcolsep}{0pt}\begin{tabular}{c} \end{tabular}}%
\psfrag{s14}[][]{\fontsize{10}{15}\fontseries{m}\mathversion{normal}\fontshape{n}\selectfont \color[rgb]{0,0,0}\setlength{\tabcolsep}{0pt}\begin{tabular}{c} \end{tabular}}%
%
% axes font properties:
\fontsize{8}{12}\fontseries{m}\mathversion{normal}%
\fontshape{n}\selectfont%
%
% xticklabels:
\psfrag{x01}[t][t]{21}%
\psfrag{x02}[t][t]{22}%
\psfrag{x03}[t][t]{23}%
\psfrag{x04}[t][t]{24}%
\psfrag{x05}[t][t]{25}%
\psfrag{x06}[t][t]{26}%
\psfrag{x07}[t][t]{27}%
\psfrag{x08}[t][t]{28}%
%
% yticklabels:
\psfrag{v01}[r][r]{1}%
\psfrag{v02}[r][r]{1.05}%
\psfrag{v03}[r][r]{1.1}%
\psfrag{v04}[r][r]{1.15}%
\psfrag{v05}[r][r]{1.2}%
\psfrag{v06}[r][r]{1.25}%
\psfrag{v07}[r][r]{1.3}%
\psfrag{v08}[r][r]{1.35}%
%
% Figure:
\resizebox{8cm}{!}{\includegraphics{ha_Alpha_1_2_3_4_5_6.matlab.eps}}%
\end{psfrags}%
%
% End ha_Alpha_1_2_3_4_5_6.matlab.tex

%\caption{Shape factor $\alpha$ for varying height and angle, $\lambda=1$. For thick, collisional flows the value quickly approaches $5/4$, indicating Bagnold velocity profiles. Values predicted for Bagnold velocity profiles ($\alpha=5/4$) and linear velocity profiles ($\alpha=3/2$) are indicated.
%\\Bottom: Shape factor $\alpha$ for varying angle and roughness, height $H=30$. The shape factor is lower for increasing smoothness.
%}
\caption{Shape factor $\alpha$ for thick, steady flow at $H=30,40$ for varying inclination $\theta$ and roughness $\lambda$. Mean values for $24^\circ\leq\theta\leq 28^\circ$ are shown as dashed lines. For thick, collisional flows over a rough base, the value quickly approaches $5/4$, indicating Bagnold velocity profiles (solid line). For smoother bases, the velocity profile becomes more convex; for $\lambda=1/2$ and high inclinations, slip can be observed; for $\lambda=0$ plug flow (dashed line) is reached. For thinner flow, the shape becomes less convex and can even be concave. 
%\todo{fix legend}
%\todo{plot the limiting case as velocity profile}
%\\Bottom: Shape factor $\alpha$ for varying angle and roughness, height $H=30$. The shape factor is lower for increasing smoothness.
}
\label{fig:alpha}
\end{figure} 

We will now take a look at the the parameters $\alpha$, $K$, and $\bar\rho$ of the depth averaged equations. We will only consider DPM simulations in which we have observed steady unordered uniform flow. 

%~ For depth-averaged values we use the density as the weighing function
%~ \begin{equation}\label{1.1}
%~ \overline{\langle\chi\rangle_w^T}= \int_\mathbb{R} \langle\chi\rangle_w^T \rho \rd z\bigg/\int_\mathbb{R} \rho \rd z.
%~ \end{equation}
%~ In the remainder of this paper the brackets are omitted and we simply write $\chi(z)=\langle\chi\rangle_w^T (z)$ and $\bar\chi=\overline{\langle\chi\rangle_w^T}$.

%In this section, the assumptions of depth-averaging are investigated. We take a look at the particle volume fraction, the flow velocity profile, and the anisotropy of the stress.
%The nearly constant density profile, apart from the microscopic layering, in Figure \ref{fig:w_dependence_nu} can be observed for all steady flow cases. 

Figure \ref{fig:Nu} shows the mean particle volume fraction $\bar\rho/\rho_p$ for varying height, inclination and roughness. The graph \linebreak[4] shows a relatively consistent collapse of the data when plotted over the inclination $\theta$. However, the mean density decreases slightly with decreasing height, and we see a marked\-ly lower density for thin flows at $H=10$, which is not shown in the graph. This might be due to the fact that the basal flow layer, which has a slightly lower density, dominates in thin flows. Indeed, plotting the mean bulk density in the center of the flow, $\rho_c=2/h\int_{h/4}^{3h/4}\rho(z)\,dz$, the data collapses onto a single curve with no obvious dependence on the height. As the inclination decreases, the mean density approaches a value of loose random packing, which can also be found in static piles below $h_s$. 

Secondly, we take a look at the shape factor $\alpha=\bar{u}^2/\overline{u^2}$ in Figure \ref{fig:alpha}. For rough bases, and at flow heights and inclinations that are sufficiently far from $h_s$, a Bagnold velocity profile, 
\begin{equation}
u(z)=\frac{5}{3}\bar{u} \left(1-\left(\frac{h-z}{h}\right)^{3/2}\right),
\end{equation}
develops, which corresponds to a shape factor of $\alpha=4/3$. For smaller base roughness the profiles collapse onto a more convex shape and thus $\alpha$ decreases; for $\lambda=0$, we even observe plug flow. Thus, $\alpha$ only depends on the basal roughness for thick, collisional flows; taking the mean values for $24^\circ\leq\theta\leq 28^\circ$, $H>30$ we obtain the following values:
$$
\begin{array}{r|r|r|r|r|r|r}
\lambda & 0 & 1/2 & 2/6 & 5/6 & 1 & 2 \\\hline
\alpha & 1.0065 & 1.1382 & 1.1986 & 1.2429 & 1.2551 & 1.2751\\\hline
\text{var}\cdot10^5 & 0.4 & 55 & 1.1 & 4.2 & 4.8 & 4.7
\end{array}
$$
where the last line denotes the standard error.
However, for thin flow or small inclinations, the flow profiles become more convex and the shape factor increases. In this case, the dependence of $\alpha$ on height and flow velocity is less obvious; we can however interpolate the values found from DPM simulations to obtain closure.

%The final important assumption is that the flow is lithostatic, \emph{i.e.} balances the gravitational forces acting on the flow; this is shown exemplary in Figure \ref{fig:K}. The fact that the flow profile is hydrostatic and the density is approximately constant allows us to approximate the downward normal stress component, as a linear function, $\sigma_{zz}^\text{lin}(z)=b-az$; we use this to define the base $b$ and surface $s$ as $\sigma_{zz}^\text{lin}(b)=\int_\mathbb{R} \rho\,dz g\cos\theta$ and  $\sigma_{zz}^\text{lin}(s)=0$, respectively.

Thirdly, the normal stress difference $K=\bar\sigma_{xx}/\bar\sigma_{zz}$ is discussed, which describes the anisotropy of the stress tensor and is expected to be unity under isotropic conditions. The range of anisotropy for steady unordered flow is generally small, ranging from 0.98 to 1.07, except for $\lambda=0$, where it can be as low as 0.68, and for the layered steady flow, as shown in Figure \ref{fig:K}. There is no clear functional dependence of $K$; however, the stress anisotropy generally increases with inclination and can roughly be fitted linearly. This behaviour is observed for all roughnesses $\lambda$.
%\todo{what about $\lambda=0$?}
Very large normal stress differences can be observed for the steady layered flow, see Figure \ref{fig:K}; these can again be fitted to a linear function of $\theta$ the layered flow.

All parameters $\bar\rho$, $\alpha$, $K$ show a functional dependence on the inclination $\theta$, and to some degree the height. The inclination $\theta$ in turn can be written as a function of the friction coefficient $\mu$ such that $\theta=\tan^{-1}(\mu(h,\bar{u}))$.  This allows us to describe the parameters of the shallow layer model in terms of the height $h$, roughness $\lambda$, and friction $\mu(h,\bar{u})$ and thus provides a proper closure for the system. For thick, collisional flows, the shape factor only depends on the basal roughness; the mean density varies only with inclination; and the normal stress anisotropy depends on roughness and inclination. For thin flows and small  inclinations, these dependencies are less clear and we need to interpolate the values found from DPM simulations to close the model. This is done for all steady unordered flows by fitting all values of $\bar\rho$ and $\alpha$ by a quadratic function of height and inclination and $K$ by a linear function, with the results shown in Table \ref{tab:fittingfull}. The values were expanded about $h=40$ and $\theta=28^\circ$ for better reading.
%\todo{It remains to be determined how well these dependencies can be used to model non-uniform flow }
%\todo{more positive, Pouliquen inertial parameter}.

\begin{figure}[tbp]
% generated by laprint.m
%
\begin{psfrags}%
\psfragscanon%
%
% text strings:
\psfrag{s01}[t][t]{\fontsize{10}{15}\fontseries{m}\mathversion{normal}\fontshape{n}\selectfont \color[rgb]{0,0,0}\setlength{\tabcolsep}{0pt}\begin{tabular}{c}$\theta$\end{tabular}}%
\psfrag{s02}[b][b]{\fontsize{10}{15}\fontseries{m}\mathversion{normal}\fontshape{n}\selectfont \color[rgb]{0,0,0}\setlength{\tabcolsep}{0pt}\begin{tabular}{c}$K$\end{tabular}}%
\psfrag{s03}[b][b]{\fontsize{10}{15}\fontseries{m}\mathversion{normal}\fontshape{n}\selectfont \color[rgb]{0,0,0}\setlength{\tabcolsep}{0pt}\begin{tabular}{c}$\lambda=1$\end{tabular}}%
\psfrag{s04}[t][t]{\fontsize{10}{15}\fontseries{m}\mathversion{normal}\fontshape{n}\selectfont \color[rgb]{0,0,0}\setlength{\tabcolsep}{0pt}\begin{tabular}{c}$\theta$\end{tabular}}%
\psfrag{s05}[b][b]{\fontsize{10}{15}\fontseries{m}\mathversion{normal}\fontshape{n}\selectfont \color[rgb]{0,0,0}\setlength{\tabcolsep}{0pt}\begin{tabular}{c}$K$\end{tabular}}%
\psfrag{s06}[b][b]{\fontsize{10}{15}\fontseries{m}\mathversion{normal}\fontshape{n}\selectfont \color[rgb]{0,0,0}\setlength{\tabcolsep}{0pt}\begin{tabular}{c}$\lambda=1/2$\end{tabular}}%
%
% axes font properties:
\fontsize{10}{15}\fontseries{m}\mathversion{normal}%
\fontshape{n}\selectfont%
%
% xticklabels:
\psfrag{x01}[t][t]{20}%
\psfrag{x02}[t][t]{22}%
\psfrag{x03}[t][t]{24}%
\psfrag{x04}[t][t]{26}%
\psfrag{x05}[t][t]{28}%
\psfrag{x06}[t][t]{20}%
\psfrag{x07}[t][t]{22}%
\psfrag{x08}[t][t]{24}%
\psfrag{x09}[t][t]{26}%
\psfrag{x10}[t][t]{28}%
%
% yticklabels:
\psfrag{v01}[r][r]{0.6}%
\psfrag{v02}[r][r]{0.7}%
\psfrag{v03}[r][r]{0.8}%
\psfrag{v04}[r][r]{0.9}%
\psfrag{v05}[r][r]{1}%
\psfrag{v06}[r][r]{1.1}%
\psfrag{v07}[r][r]{1.2}%
\psfrag{v08}[r][r]{1.3}%
\psfrag{v09}[r][r]{0.99}%
\psfrag{v10}[r][r]{1}%
\psfrag{v11}[r][r]{1.01}%
\psfrag{v12}[r][r]{1.02}%
\psfrag{v13}[r][r]{1.03}%
\psfrag{v14}[r][r]{1.04}%
\psfrag{v15}[r][r]{1.05}%
%
% Figure:
\resizebox{8cm}{!}{\includegraphics{ha_K_5_2.matlab.eps}}%
\end{psfrags}%
%
% End ha_K_5_2.matlab.tex

%\input{FiguresMatlab/ha_K_5.matlab.tex}
\caption{Normal stress difference $K=\bar\sigma_{xx}/\bar\sigma_{zz}$ for varying height $H=20$, 30, 40 and inclination and $\lambda=1$ (left), resp. $\lambda=1/2$ (right). Markers denote steady $\circ$, layered $\times$, and oscillating $\diamond$ flow. Lines denote linear fits of the steady and layered flows; for $\lambda=1$.}
\label{fig:K}
\end{figure}

\begin{table*}[tbp]
$$\begin{array}{|r|r|r|r|r|r|r|r|r|r|r|r|}\hline
\lambda & c_0 & c_1 & c_2 & c_3 & \text{var}\\\hline
0 & 0.718087 & 1.873696 & 0.151112 & 0.750073 &0.025\\
1/2 & 0.559997 & 0.083827 & 0.686181 & 0.952036 &0.007\\
2/3 & 0.589451 & 0.084660 & 0.319469 & 0.435792 &0.003\\
5/6 & 0.596186 & 0.061257 & 0.259384 & 0.252192 &0.002\\
1 & 0.595057 & 0.061628 & 0.249987 & 0.254915 &0.001\\
2 & 0.608831 & 0.155089 & 0.166334 & 0.384397 &0.003\\
\hline\end{array}
\quad
\begin{array}{|r|r|r|r|r|r|r|r|r|r|r|r|}\hline
\lambda & c_4 & c_5 & c_6 & \text{var}\\\hline
0 & 1.016654 & & &0.016\\
1/2 & 1.144799 & & &0.016\\
2/3 & 1.182573 & 1.072630 & 0.144773 &0.010\\
5/6 & 1.235808 & 2.776600 & 0.301505 &0.009\\
1 & 1.231833 & 2.526435 & 0.182988 &0.008\\
2 & 1.223064 & 4.396744 & 0.143197 &0.024\\
\hline\end{array}
\quad
\begin{array}{|r|r|r|r|r|r|r|r|r|r|r|r|}\hline
\lambda & c_7 & c_8 & \text{var}\\\hline
0 & 1.003536 & 0.044403 &0.089\\
1/2 & 1.001288 & 0.011794 &0.008\\
2/3 & 1.012662 & 0.008015 &0.005\\
5/6 & 1.022136 & 0.007245 &0.016\\
1 & 1.018992 & 0.008194 &0.010\\
2 & 1.023099 & 0.007853 &0.016\\
\hline\end{array}$$

\caption{Fittings for the mean density$\bar\rho(\theta,h)=c_0-c_1\exp(c_2(\theta-24^\circ)/1^\circ)/h^{c_3}$, the shape factor $\alpha(\theta,h)=c_4+c_5\exp(-c_6(\theta-\theta_s(h))/1^\circ)/h$, and the stress anisotropy $K(\theta,h)=c_7+c_8(\theta-24^\circ)/1^\circ$. $\text{var}$ denotes the variance of the difference between measured and fitted values. Closure relations are fitted to all data sets of steady unordered flow, $\delta_3^\lambda<\theta\leq\delta_{acc}^\lambda$.}
\label{tab:fittingfull}
\end{table*}

\begin{figure*}[tbp]
\centering
% generated by laprint.m
%
\begin{psfrags}%
\psfragscanon%
%
% text strings:
\psfrag{s01}[t][t]{\fontsize{10}{15}\fontseries{m}\mathversion{normal}\fontshape{n}\selectfont \color[rgb]{0,0,0}\setlength{\tabcolsep}{0pt}\begin{tabular}{c}$\theta$\end{tabular}}%
\psfrag{s02}[b][b]{\fontsize{10}{15}\fontseries{m}\mathversion{normal}\fontshape{n}\selectfont \color[rgb]{0,0,0}\setlength{\tabcolsep}{0pt}\begin{tabular}{c}$\bar\rho$\end{tabular}}%
\psfrag{s05}[l][l]{\fontsize{10}{15}\fontseries{m}\mathversion{normal}\fontshape{n}\selectfont \color[rgb]{0,0,0}$H=10$}%
\psfrag{s06}[l][l]{\fontsize{10}{15}\fontseries{m}\mathversion{normal}\fontshape{n}\selectfont \color[rgb]{0,0,0}$H=40$}%
\psfrag{s07}[l][l]{\fontsize{10}{15}\fontseries{m}\mathversion{normal}\fontshape{n}\selectfont \color[rgb]{0,0,0}$H=30$}%
\psfrag{s08}[l][l]{\fontsize{10}{15}\fontseries{m}\mathversion{normal}\fontshape{n}\selectfont \color[rgb]{0,0,0}$H=20$}%
\psfrag{s09}[l][l]{\fontsize{10}{15}\fontseries{m}\mathversion{normal}\fontshape{n}\selectfont \color[rgb]{0,0,0}$H=10$}%
\psfrag{s11}[t][t]{\fontsize{10}{15}\fontseries{m}\mathversion{normal}\fontshape{n}\selectfont \color[rgb]{0,0,0}\setlength{\tabcolsep}{0pt}\begin{tabular}{c}$\theta$\end{tabular}}%
\psfrag{s12}[b][b]{\fontsize{10}{15}\fontseries{m}\mathversion{normal}\fontshape{n}\selectfont \color[rgb]{0,0,0}\setlength{\tabcolsep}{0pt}\begin{tabular}{c}$\alpha$\end{tabular}}%
\psfrag{s15}[][]{\fontsize{10}{15}\fontseries{m}\mathversion{normal}\fontshape{n}\selectfont \color[rgb]{0,0,0}\setlength{\tabcolsep}{0pt}\begin{tabular}{c} \end{tabular}}%
\psfrag{s16}[][]{\fontsize{10}{15}\fontseries{m}\mathversion{normal}\fontshape{n}\selectfont \color[rgb]{0,0,0}\setlength{\tabcolsep}{0pt}\begin{tabular}{c} \end{tabular}}%
\psfrag{s17}[t][t]{\fontsize{10}{15}\fontseries{m}\mathversion{normal}\fontshape{n}\selectfont \color[rgb]{0,0,0}\setlength{\tabcolsep}{0pt}\begin{tabular}{c}$\theta$\end{tabular}}%
\psfrag{s18}[b][b]{\fontsize{10}{15}\fontseries{m}\mathversion{normal}\fontshape{n}\selectfont \color[rgb]{0,0,0}\setlength{\tabcolsep}{0pt}\begin{tabular}{c}$K$\end{tabular}}%
%
% axes font properties:
\fontsize{10}{15}\fontseries{m}\mathversion{normal}%
\fontshape{n}\selectfont%
%
% xticklabels:
\psfrag{x01}[t][t]{20}%
\psfrag{x02}[t][t]{22}%
\psfrag{x03}[t][t]{24}%
\psfrag{x04}[t][t]{26}%
\psfrag{x05}[t][t]{28}%
\psfrag{x06}[t][t]{22}%
\psfrag{x07}[t][t]{24}%
\psfrag{x08}[t][t]{26}%
\psfrag{x09}[t][t]{28}%
\psfrag{x10}[t][t]{22}%
\psfrag{x11}[t][t]{24}%
\psfrag{x12}[t][t]{26}%
\psfrag{x13}[t][t]{28}%
%
% yticklabels:
\psfrag{v01}[r][r]{0.99}%
\psfrag{v02}[r][r]{1}%
\psfrag{v03}[r][r]{1.01}%
\psfrag{v04}[r][r]{1.02}%
\psfrag{v05}[r][r]{1.03}%
\psfrag{v06}[r][r]{1.04}%
\psfrag{v07}[r][r]{1.05}%
\psfrag{v08}[r][r]{1.25}%
\psfrag{v09}[r][r]{1.3}%
\psfrag{v10}[r][r]{1.35}%
\psfrag{v11}[r][r]{1.4}%
\psfrag{v12}[r][r]{1.45}%
\psfrag{v13}[r][r]{0.51}%
\psfrag{v14}[r][r]{0.52}%
\psfrag{v15}[r][r]{0.53}%
\psfrag{v16}[r][r]{0.54}%
\psfrag{v17}[r][r]{0.55}%
\psfrag{v18}[r][r]{0.56}%
\psfrag{v19}[r][r]{0.57}%
\psfrag{v20}[r][r]{0.58}%
%
% Figure:
\resizebox{16cm}{!}{\includegraphics{table_fittingfull5.matlab.eps}}%
\end{psfrags}%
%
% End table_fittingfull5.matlab.tex

%\input{FiguresMatlab/ha_K_5.matlab.tex}
\caption{Mean density, shape factor, and stress anisotropy for rough base, $\lambda=1$. Markers denote the DPM data, lines the values fitted according to Table \ref{tab:fittingfull}.}
\label{fig:fittingfull}
\end{figure*}
